# Supplementary material for: Knowledge Evolution in Neural Networks
Source: arXiv:2103.05152 source file (2021-03-09)
Supplement: Supplementary file 1 [file 5385_ke_supp.tex]

% This version of CVPR template is provided by Ming-Ming Cheng.
% Please leave an issue if you found a bug:
% https://github.com/MCG-NKU/CVPR_Template.

\documentclass[review]{cvpr}

\usepackage{times}
\usepackage{epsfig}
\usepackage{graphicx}
\usepackage{amsmath}
\usepackage{amssymb}

\usepackage{multirow}
\usepackage{comment}
\usepackage{xcolor,colortbl} 
\usepackage{soul}

\usepackage[ruled,vlined,linesnumbered]{algorithm2e}
\usepackage[abbreviations]{foreign}
\usepackage{enumitem}

\usepackage{bm}
\usepackage{dsfont}

\makeatletter
\@namedef{ver@everyshi.sty}{}
\makeatother
\usepackage{tikz}
\usepackage{pgfplots}
\usetikzlibrary{pgfplots.groupplots}
\usepgfplotslibrary{groupplots}

\usepackage{fp}
\usepackage{xfp}

\usepackage{multicol}
\usepackage{booktabs}       % professional-quality tables

\usepackage{array}
\newcolumntype{H}{>{\setbox0=\hbox\bgroup}c<{\egroup}@{}}

% Include other packages here, before hyperref.

% If you comment hyperref and then uncomment it, you should delete
% egpaper.aux before re-running latex.  (Or just hit 'q' on the first latex
% run, let it finish, and you should be clear).
\usepackage[pagebackref=true,breaklinks=true,colorlinks,bookmarks=false,citecolor=blue]{hyperref}

\usepackage[numbers]{natbib}

\begin{comment} ## up comment for proof reading. 
\usepackage{environ}
\RenewEnviron{figure*}{}
\RenewEnviron{figure}{}

\RenewEnviron{table}{}
\RenewEnviron{table*}{}
\RenewEnviron{algorithm}{}
\RenewEnviron{equation}{}
\RenewEnviron{align}{}

\end{comment}

 % *** Enter the CVPR Paper ID here

%\setcounter{page}{4321} % For final version only

\newcommand*{\rom}[1]{\uppercase\expandafter{\romannumeral #1\relax}}

\begin{document}

%%%%%%%%% TITLE
\title{Knowledge Evolution in Neural Networks \\ Appendix}
%\title{Paper Title}

\author{Ahmed Taha ~\etal\\
University of Maryland\\
%Institution1 address\\
%{\tt\small firstauthor@i1.org}
% For a paper whose authors are all at the same institution,
% omit the following lines up until the closing ``}''.
% Additional authors and addresses can be added with ``\and'',
% just like the second author.
% To save space, use either the email address or home page, not both
%\and
%Second Author\\
%Institution2\\
%First line of institution2 address\\
%{\tt\small secondauthor@i2.org}
}

\maketitle

\appendix
\section{Appendix}
\input{supp_mat}

{\small
	\bibliographystyle{ieee_fullname}
	\bibliography{split_nets}
}

\end{document}
