# Supplementary material for: Knowledge Evolution in Neural Networks
Source: arXiv:2103.05152 source file (2021-03-09)
Supplement: Supplementary file 2 [file split_nets_supp.tex]

\documentclass[review]{cvpr}

\usepackage{times}
\usepackage{epsfig}
\usepackage{graphicx}
\usepackage{amsmath}
\usepackage{amssymb}

\usepackage{breqn}

\usepackage{multirow}
\usepackage{comment}
\usepackage{xcolor,colortbl} 

\usepackage[ruled,vlined,linesnumbered]{algorithm2e}

\usepackage[abbreviations]{foreign}
\usepackage{enumitem}

\usepackage{bm}

\makeatletter
\@namedef{ver@everyshi.sty}{}
\makeatother
\usepackage{tikz}
\usepackage{pgfplots}
\usetikzlibrary{pgfplots.groupplots}
\usepgfplotslibrary{groupplots}

\usepackage{fp}
\usepackage{xfp}

\usepackage{multicol}
\usepackage{booktabs}       % professional-quality tables

% Include other packages here, before hyperref.

% If you comment hyperref and then uncomment it, you should delete
% egpaper.aux before re-running latex.  (Or just hit 'q' on the first latex
% run, let it finish, and you should be clear).
\usepackage[pagebackref=true,breaklinks=true,letterpaper=true,colorlinks,bookmarks=false]{hyperref}

 % *** Enter the CVPR Paper ID here

%\renewcommand{\tableautorefname}{Tab.}

\newcommand*{\rom}[1]{\uppercase\expandafter{\romannumeral #1\relax}}

\begin{document}

%%%%%%%%% TITLE
\title{Knowledge Evolution in Neural Networks}

\author{First Author\\
Institution1\\
Institution1 address\\
{\tt\small firstauthor@i1.org}
% For a paper whose authors are all at the same institution,
% omit the following lines up until the closing ``}''.
% Additional authors and addresses can be added with ``\and'',
% just like the second author.
% To save space, use either the email address or home page, not both
\and
Second Author\\
Institution2\\
First line of institution2 address\\
{\tt\small secondauthor@i2.org}
}

\maketitle

\newcommand{\beginsupplement}{%
	\setcounter{table}{0}
	\renewcommand{\thetable}{A\arabic{table}}%
	\setcounter{figure}{0}
	\renewcommand{\thefigure}{A\arabic{figure}}%
	\setcounter{section}{0}
	\renewcommand{\thesection}{A\arabic{section}}%
	\setcounter{equation}{0}
	\renewcommand{\theequation}{A\arabic{equation}}%
}

\beginsupplement

\input{supp_mat}
{\small
\bibliographystyle{ieee_fullname}
\bibliography{tm_inf}
}

\end{document}
