# Supplementary material for: Knowledge Evolution in Neural Networks
Source: arXiv:2103.05152 source file (2021-03-09)
Supplement: Supplementary file 3 [file old_supp_mat.tex]

The following appendix sections extend their corresponding sections in the main paper. For instance, the related-work appendix~\ref{sec:app_related} extends the related-work section in the main paper.

\appendix

%\section{Further Comments}
\section{Appendix: Related Work}\label{sec:app_related}
\begin{enumerate}
	\item Lottery Ticket hypothesis literature~\cite{frankle2018lottery,zhou2019deconstructing,frankle2019stabilizing}. Both~\cite{frankle2018lottery,zhou2019deconstructing} study the lottery ticket hypothesis on small datasets. In this literature,  the lottery ticket subnetwork is always reset to its randomly initialized weights -- $W$ at iteration zero. Frankle~\etal~\cite{frankle2019stabilizing} showed that this strict weight resetting harms performance on large scale datasets. Accordingly, weight rewinding~\cite{frankle2019stabilizing} is proposed, which 
	rewinds pruned subnetwork's weights to their former values at iteration $k$ rather than resetting them to iteration zero.
	These three papers~\cite{frankle2018lottery,zhou2019deconstructing,frankle2019stabilizing} are solving a network pruning problem. Thus, the pruned network performance is always less than or equal to the dense network. This is not the case for Task-Mask. 
	
	%\item Supermask literature~\cite{wortsman2020supermasks,ramanujan2020s}
	%\item Network initialization literature~\cite{glorot2010understanding,krahenbuhl2015data} initializes each layer independently.
	
%	\item Born again neural networks~\cite{furlanello2018born} assume a teacher model with access to a large corps of data, Task-Mask does not. In born-again, every student uses the predictions of the previous teacher model to distill knowledge, Task-Mask does not. In born-again, students are randomly initialized, Task-Mask does not.
	%	\item Our work can be regarded a a generalization of the Dense-Sparse-Dense (DSD) training protocol~\cite{han2016dsd}. Yet, there are technical and non-technical factors that differentiate our work. The technical factors are clear; 
	
	%\item SOTA on small datasets~\cite{yun2020regularizing}. Baselines: AdaCos~\cite{zhang2019adacos}, Virtual-softmax~\cite{chen2018virtual}, Maximum-entropy~\cite{dubey2018maximum,pereyra2017regularizing}, Label-smoothing~\cite{muller2019does,szegedy2016rethinking} , DDGSD~\cite{xu2019data}, BYOT~\cite{zhang2019your}
	%\item The argument that pre-trained networks~\cite{erhan2010does} and knowledge distillation~\cite{yuan2020revisiting} are just regularizers. Similarly, Task-Mask can be regarded as a weight-regularizer.
	%\item Few-show learning approaches~\cite{bateni2020improved,requeima2019fast} count on pretrained ImageNet weights~\cite{deng2009imagenet}, Task-Mask do not.
	%\item I should cite some evolutionary machine learning literature.
\end{enumerate}

\section{Appendix: Approach}
\begin{equation}
{ M }_{ l+1 }^{ w,h,j }=\sum _{ i=1 }^{ C_{ i } }{ \sum _{ c=1 }^{ \kappa  }{ \sum _{ r=1 }^{ \kappa  }{ 
			{ w }_{ ji }^{ (c,r) }{ M }_{ l }^{ \left( w+c-\left\lceil \frac { \kappa  }{ 2 }  \right\rceil ,h+r-\left\lceil \frac { \kappa  }{ 2 }  \right\rceil ,i \right)  } 
}  }  } 
\end{equation}
%where $\Psi_i  = { w }_{ ji }^{ (c,r) }{ M }_{ l }^{ \left( w+c-\left\lceil \frac { \kappa  }{ 2 }  \right\rceil ,h+r-\left\lceil \frac { \kappa  }{ 2 }  \right\rceil ,i \right)  } $


\begin{equation}
{ M }_{ l+1 }^{ w,h,j }=\sum _{ i=1 }^{ C_{ i } }{ \sum _{ c=1 }^{ \kappa  }{ \sum _{ r=1 }^{ \kappa  }{ { w }_{ ji }^{ (c,r) }{ M }_{ l }^{ \left( w+c-\left\lceil \frac { \kappa  }{ 2 }  \right\rceil ,h+r-\left\lceil \frac { \kappa  }{ 2 }  \right\rceil ,i \right)  } }  } h\left( { s }_{ l }^{ j } \right)  } 
\end{equation}

\begin{equation}
{ s }_{ l }^{ j }\leftarrow { s }_{ l }^{ j }-lr\sum _{ i=1 }^{ C_{ i } }{ \sum _{ w=1 }^{ W }{ \sum _{ h=1 }^{ H }{ \sum _{ c=1 }^{ \kappa  }{ \sum _{ r=1 }^{ \kappa  }{ \frac { \partial L }{ \partial { M }_{ l+1 }^{ w,h,j } } { w }_{ ji }^{ (c,r) }{ M }_{ l }^{ \left( w+c-\left\lceil \frac { \kappa  }{ 2 }  \right\rceil ,h+r-\left\lceil \frac { \kappa  }{ 2 }  \right\rceil ,i \right)  } }  }  }  }  } 
\end{equation}


\begin{figure*}
	\centering
	\includegraphics[width=1.0\linewidth]{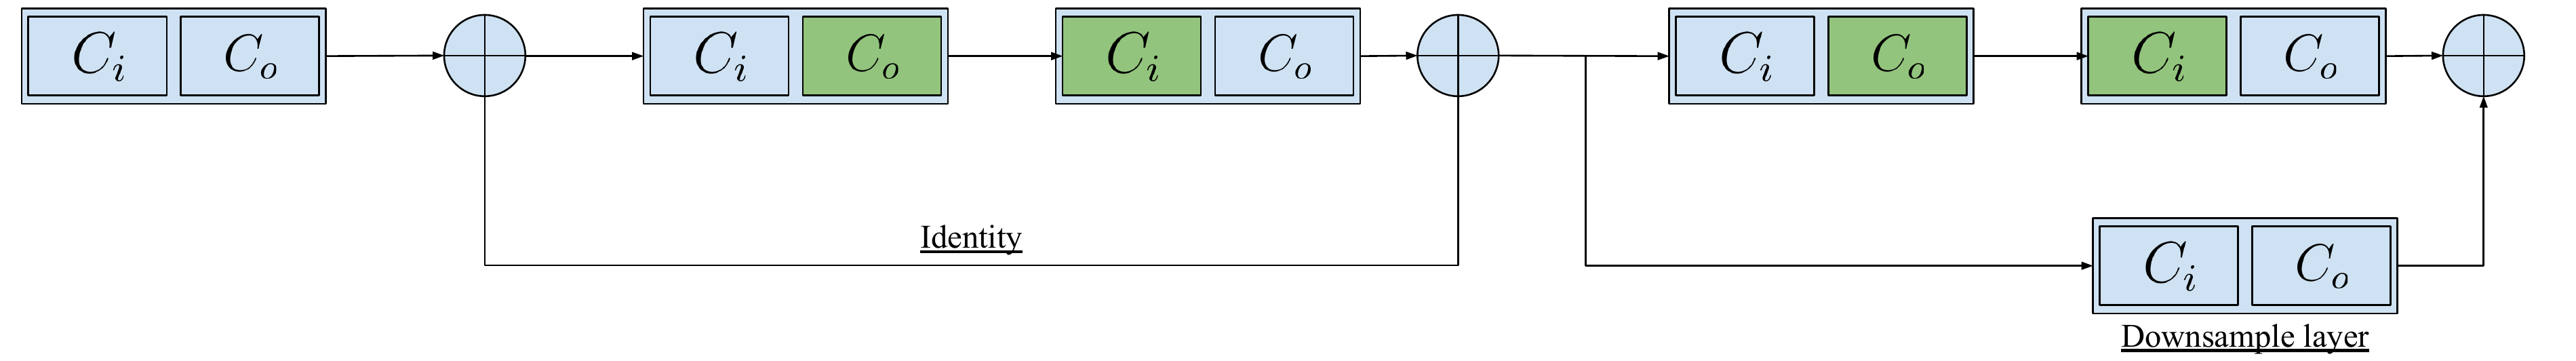}
	\caption{A simple approach to convert a toy residual network into a slim residual network. We prune the output filters and the corresponding input channels highlighted in green. We omit the RELU and batch norm layers for brevity; However, they will be pruned as well. This simple approach will keep a lot of filters set to zero, to  add feature maps properly. Yet, the computational reduction during inference remains significant.}
	\label{fig:simplepruning}
\end{figure*}


\section{Appendix:  Experiments}

\heading{TM vs RePr:} In the paper, we highlight two differences between TM and RePr. Yet, there are other worth nothing differences. (\rom{1}) TM uses popup scores to quantify each filter's importance. Our ablation study (Figure~\ref{}) emphasizes the importance of \textbf{re-using} these scores across different mask phases. Basically, TM is biased towards filters (hypotheses) that survived previous mask phases. This achieves superior performance, compared to resetting the scores and re-ranking filters from scratch. However, RePr ranks filters from scratch at every pruning stage. This is an inferior ranking policy.

(\rom{2}) RePr and TM also differ in terms of the final network sparsity. Since RePr is a training approach for large datasets, RePr terminates with a dense network. In contrast, TM is a training approach for small datasets. Thus, TM is able to deliver both a sparse and dense networks (Figure~\ref{}) due to the redundancy in deep networks' trained on small datasets.

%For example, If the probably of a filter being redundant is $p$ at the first pruning stage, 
 
% does not have an equivalent 



\subsection{Interesting Ablation Studies}
I am looking forward to the following set of experiments

\begin{enumerate}
	\item Can the knowledge accumulated from a single dataset transfer to a different dataset? For instance, If I train 100 generations on Flower102, how do these generations perform on CUB-200?
	\item Apply Task-Mask on feature embedding networks. To my knowledge, Task-Mask would be the first approach  that boosts \textit{both} classification and feature embedding networks on small datasets.
	\item How do the filters of the first conv layer look like? When pretrained on ImageNet, the filters of the first conv layer look like edge detectors. Can Task-Mask learn similar filters from a small dataset? This would be a sign for generalization beyond the small dataset used during evolution.
	\item In this paper, I am going to focus on supervised tasks only. However, investigation on unsupervised tasks is an interesting future extension. 
	
	\item Typical regularization approaches fail as the trained network becomes deeper. Task-Mask approach fails if and only if the dataset gets bigger while the network size remains fixed or decreases. As the network-size gets bigger, task-mask should remain competitive. Assuming a fixed pruning rate, as the network becomes bigger, the number of possible subnetworks increases. The Mask-phase, having a large diversity in weights, will locate better fit-weights which speed up the performance progress. 
	
	%However, it is the opposite for Task-Mask.  
\end{enumerate}

The following is a set of ablation studies that I am *not* looking for, but I should do

\begin{enumerate}
	\item Does a better sampling distribution $D$ exist? I expect a sampling strategy that takes the weight magnitude into account to be better~\cite{zhou2019deconstructing}. However, the anticipated improvement will not justify the added complexity. 
	\item The reason I am not identifying fit-bias is that (1) I do not think bias terms correlate across layers, (2) the bias term reflects how a network favors or thwarts classes against each other.  Bias is a way to define a threshold between classes, it reflects the distribution of the input classes; majority classes have bigger bias terms while minority classes have a smaller bias. Accordingly, there is no bad and fit-bias to transfer. I should show empirically that transfer fit-bias brings no improvement.
\end{enumerate}



\subsection{Misc Notes}
\begin{enumerate}
	\item The \textit{current} main limitation of Task-Mask is the computational complexity during training. For a single dataset, the \textit{current} Task-Mask approach trains $2 \times G$ neural networks,~\ie $G$ tasks and $G$ masks networks. At this preliminary stage, I intentionally did not pay attention to this issue because I wanted to focus more on the approach and the SOTA performance even if it is computationally costly. It is important to note that one epoch of ImageNet is computationally equivalent to one thousand epochs of Flower102. I am not promising anything, but I will think about how to reduce the training cost in the upcoming stage. 
	% For a small dataset, this is not a huge issue. 
	
	\item There is an expected argument that this approach is not valuable for big datasets. While this argument is expected, I think it is a shortsighted one. In less than a decade, the size of neural networks will grow very big~\cite{brown2020language}. If ImageNet is currently enough to train a deep network, it won't be in the future -- it will become a toy dataset. Of course, self/un-supervised approaches do not need labels, yet they need a ton of unlabeled data. This is not a feasible solution for applications such as autonomous navigation, medical imaging, and any application with privacy concerns. 
	
	\item The killing argument is, why not use ImageNet weights, instead of random weights? The best reply is to show that Task-Mask boosts the performance of networks initialized with either random or ImageNet weights. Maybe it will, I am not sure! More experiments are needed to address this argument.
	
	%I think it is better if I presented Task-Mask not as an approach for small datasets, but as an approach for labeled datasets on very deep neural networks. But, I can not train any very deep neural network on vulcan!
	
	\item Task-Mask integrates seamlessly with all neural network training tricks.  I should capitalize on this strength in my experiments. For example, I am currently using cross entropy with the label smoothing regularizer, but I can also use the SOTA class-wise regularizer~\cite{yun2020regularizing}.
	
	
	% I a presented Task-Mask approach as a solution to train a relatively deep network on a relatively small tasks -- not an absolute small.
\end{enumerate}

\begin{table}[]
	\scriptsize
	\begin{tabular}{lll}
		\toprule
		Layers                & Dense  $N$                       & Fit-hypothesis $H^\triangle$ ($s_r=0.5$)          \\
		
		\midrule
		conv1                             & 64 $\times$ 7 $\times$ 7 $\times$ 3    & 32 $\times$ 7 $\times$ 7 $\times$ 3    \\
		bn1                               & 64                                     & 32                                     \\
		layer1.0.conv1                    & 64 $\times$ 3 $\times$ 3 $\times$ 64   & 32 $\times$ 3 $\times$ 3 $\times$ 32   \\
		layer1.0.bn1                      & 64                                     & 32                                     \\
		layer1.0.conv2                    & 64 $\times$ 3 $\times$ 3 $\times$ 64   & 32 $\times$ 3 $\times$ 3 $\times$ 32   \\
		layer1.0.bn2                      & 64                                     & 32                                     \\
		layer1.1.conv1                    & 64 $\times$ 3 $\times$ 3 $\times$ 64   & 32 $\times$ 3 $\times$ 3 $\times$ 32   \\
		layer1.1.bn1                      & 64                                     & 32                                     \\
		layer1.1.conv2                    & 64 $\times$ 3 $\times$ 3 $\times$ 64   & 32 $\times$ 3 $\times$ 3 $\times$ 32   \\
		layer1.1.bn2                      & 64                                     & 32                                     \\
		layer2.0.conv1                    & 128 $\times$ 3 $\times$ 3 $\times$ 64  & 64 $\times$ 3 $\times$ 3 $\times$ 32   \\
		layer2.0.bn1                      & 128                                    & 64                                     \\
		layer2.0.conv2                    & 128 $\times$ 3 $\times$ 3 $\times$ 128 & 64 $\times$ 3 $\times$ 3 $\times$ 64   \\
		layer2.0.bn2                      & 128                                    & 64                                     \\
		layer2.0.downsample.0             & 128 $\times$ 1 $\times$ 1 $\times$ 64  & 64 $\times$ 1 $\times$ 1 $\times$ 32   \\
		layer2.0.downsample.1             & 128                                    & 64                                     \\
		layer2.1.conv1                    & 128 $\times$ 3 $\times$ 3 $\times$ 128 & 64 $\times$ 3 $\times$ 3 $\times$ 64   \\
		layer2.1.bn1                      & 128                                    & 64                                     \\
		layer2.1.conv2                    & 128 $\times$ 3 $\times$ 3 $\times$ 128 & 64 $\times$ 3 $\times$ 3 $\times$ 64   \\
		layer2.1.bn2                      & 128                                    & 64                                     \\
		layer3.0.conv1                    & 256 $\times$ 3 $\times$ 3 $\times$ 128 & 128 $\times$ 3 $\times$ 3 $\times$ 64  \\
		layer3.0.bn1                      & 256                                    & 128                                    \\
		layer3.0.conv2                    & 256 $\times$ 3 $\times$ 3 $\times$ 256 & 128 $\times$ 3 $\times$ 3 $\times$ 128 \\
		layer3.0.bn2                      & 256                                    & 128                                    \\
		layer3.0.downsample.0             & 256 $\times$ 1 $\times$ 1 $\times$ 128 & 128 $\times$ 1 $\times$ 1 $\times$ 64  \\
		layer3.0.downsample.1             & 256                                    & 128                                    \\
		layer3.1.conv1                    & 256 $\times$ 3 $\times$ 3 $\times$ 256 & 128 $\times$ 3 $\times$ 3 $\times$ 128 \\
		layer3.1.bn1                      & 256                                    & 128                                    \\
		layer3.1.conv2                    & 256 $\times$ 3 $\times$ 3 $\times$ 256 & 128 $\times$ 3 $\times$ 3 $\times$ 128 \\
		layer3.1.bn2                      & 256                                    & 128                                    \\
		layer4.0.conv1                    & 512 $\times$ 3 $\times$ 3 $\times$ 256 & 256 $\times$ 3 $\times$ 3 $\times$ 128 \\
		layer4.0.bn1                      & 512                                    & 256                                    \\
		layer4.0.conv2                    & 512 $\times$ 3 $\times$ 3 $\times$ 512 & 256 $\times$ 3 $\times$ 3 $\times$ 256 \\
		layer4.0.bn2                      & 512                                    & 256                                    \\
		layer4.0.downsample.0             & 512 $\times$ 1 $\times$ 1 $\times$ 256 & 256 $\times$ 1 $\times$ 1 $\times$ 128 \\
		layer4.0.downsample.1             & 512                                    & 256                                    \\
		layer4.1.conv1                    & 512 $\times$ 3 $\times$ 3 $\times$ 512 & 256 $\times$ 3 $\times$ 3 $\times$ 256 \\
		layer4.1.bn1                      & 512                                    & 256                                    \\
		layer4.1.conv2                    & 512 $\times$ 3 $\times$ 3 $\times$ 512 & 256 $\times$ 3 $\times$ 3 $\times$ 256 \\
		layer4.1.bn2                      & 512                                    & 256                                    \\
		fc                                & 102 $\times$ 512                       & 102 $\times$ 256                       \\
		\midrule
		\midrule
		\#Ops (GOps) & 3.632420  &  0.968436 \\
		\#Parameters (M) & 11.285862 &  2.853606 \\
		\bottomrule
	\end{tabular}
\end{table}
